# Supplementary material for: Best-Response Dynamics and Fictitious Play in Identical-Interest and Zero-Sum Stochastic Games
Source: arXiv:2111.04317 source file (2022-05-16)
Supplement: Supplementary file 1 [file appendix_extended_comparison.tex]

\hypertarget{app:related}{
\section{Extended Comparison with Existing Work}
\label{app:related}}

\paragraph{Fictitious play in non-stochastic normal form games}

Fictitious play was originally introduced by \citeauthor*{brown1951iterative} and \citeauthor*{robinsonIterativeMethodSolving1951} for zero-sum games. Its convergence was proven for several class of games (see \ref{sec:related} for details). Its continuous counterpart is the best-response dynamics and it was studied by numerous authors, including \cite{harrisRateConvergenceContinuousTime1998a}.

The studied games are not stochastic, so there is no state in the stochastic sense. Therefore there is only one strategy profile $x(t)$ that evolves with time $t$ according to the following differential inclusion:

\begin{equation}\label{eq:harris}
    \diff x^i \in \text{BR}^i(x^{-i})
\end{equation}

where $BR^i(x^{-i})$ is the best response of player $i$, i.e. the set of actions $a$ that maximizes $r^i(a, x^{-i}))$.

\citeauthor*{benaimStochasticApproximationsDifferential2005} showed in \cite{benaimStochasticApproximationsDifferential2005} that the limit set of discrete time fictitious play can be studied using (\ref{eq:harris}): the continuous time interpolation is a so called asymptotic pseudo-trajectory.

\citeauthor*{benaimConsistencyVanishinglySmooth2013} exhibit a simple Lyapunov function for \ref{eq:harris} in identical interest games (and more generally in potential games): $t\mapsto r^i(x(t))$ is increasing if $r^i$ is concave (in the games defined in our paper, it is linear) in every variable.

This approach can not be used as-is for stochastic games: even identical interest stochastic games do not necessarily have concave value function in every player strategy across states. Therefore, it is necessary to rely on other potential functions or other proof techniques. This approach was carried out in \cite{perkinsAdvancedStochasticApproximation2013} where the total discounted payoff of a strategy is computed at every step of the algorithm. Then, an immediate best-response is computed and played. Computing such functions across all states is potentially costly (it requires to solve the Markovian decision process). We described in our paper a procedure that does not need the whole Markovian decision process to be solved at every step.

\paragraph{Best-response dynamics in zero-sum stochastic games}
\ \newline
\citeauthor*{leslieBestresponseDynamicsZerosum2020} introduced the best-response dynamic in a zero-sum stochastic game as follows for every $s$, $i$ and $t \geq 1$:

\begin{equation}\label{eq:leslie}
    \left\{\begin{aligned}
        &\dot u_s(t)=\frac{f_{s, u(t)}(x_s(t))-u_s(t)}{t} \\
        &\dot x^i_s(t) \in \argmax{a \in A^i}f_{s, u}(a, x^{-i}_s(t))-x^i_s(t)
    \end{aligned}
    \right.
\end{equation}

Compared to our paper, their work is dedicated to zero-sum stochastic games in continuous time whereas our paper deals with identical interest stochastic games and study discrete-time fictitious play using the continuous time best-response. Therefore, it is the first time, to the best of our knowlegde, that ideas from \cite{leslieBestresponseDynamicsZerosum2020} are used in an algorithm to perform online learning.

Our paper is inspired from \cite{leslieBestresponseDynamicsZerosum2020} and as such, share many similarities, including the different learning rates for $u_s$ and $x^i_s$. In our continous time systems, the different learning rates are generalized and $u_s$ are updated at rate $\alpha(t)$, so $\alpha(t)=t$ gives (\ref{eq:leslie}).

Furthermore, a state-dependent system is also defined in \cite{leslieBestresponseDynamicsZerosum2020} as follows:

\begin{equation}\label{eq:leslie2}
    \left\{\begin{aligned}
        &\dot u_s(t)=\frac{f_{s, u(t)}(x_s(t))-u_s(t)}{t} \\
        &\dot x^i_s(t) \in 1_{s=s(t)}\left(\argmax{a \in A^i}f_{s, u}(a, x^{-i}_s(t))-x^i_s(t)\right)
    \end{aligned}
    \right.
\end{equation}

where $s(t)$ is the state at time $t$.

This corresponds to semi-asynchronous systems \ref{eq:sabrd}. However, in contrast to (\ref{eq:leslie2}), in \ref{eq:sabrd}, the update rate is at least $\beta_- > 0$ because it stands for an average over a continuous period of time. This is a different way to use the ergodicity hypothesis and it is especially well suited for our article because our goal is to prove the convergence of the discrete time systems using continuous time systems. So, the average over time is consubstantial with stochastic approximations.

We also provide fully asynchronous systems \ref{eq:abrd} where $u_s$ is also updated in a stade dependent manner, which is not the case in \cite{leslieBestresponseDynamicsZerosum2020}.

\paragraph{Fictitious play in zero-sum games}
\citeauthor*{sayinFictitiousPlayZerosum2020} introduced an algorithm that combines fictitious play and $Q$-learning in zero-sum stochastic games. It is defined with estimates of the state-action value function $\hat Q_{i, s, n}(a)$ for player $i$, state $s$, action $a$ and step $n$ of the algorithm and estimates of the other player startegies $\hat \pi_{1, s, n}$ (which is $x^i_{s,n})$ with our notations). This differ from our work in three fundamental directions. First, it is based on state-action value functions $\hat Q_{i, s, n}(a)$, whereas our work is built upon state value functions $u^i_{s, n}$. Second, the games considered are zero-sum (fully competitive) stochastic games whereas we focus on identical interest (fully cooperative) stochastic games. Third, it is technically built upon different proof techniques as \citeauthor*{sayinFictitiousPlayZerosum2020} also use stochastic approximations but the different timescale are not present in the continuous-time systems.

The update on the $Q$-function when the profile $a$ is played and the current state is $s$ at step $n$ is (for other actions, the $Q$-function is unchanged):

\optmult{\hat Q_{i, s, n}(a) = \hat Q_{i, s, n}(a) \\ + \hat \beta_{s, n}\left(r^i(s, a) + \gamma \sum_{s' \in \mathcal S}\hat v_{i, n}(s')P_{ss'}(a)-\hat Q_{i, s, n}(a)\right)}
where $\hat v_{i, n}(s') = \max_{a^i \in A^i} Q_{i, s, n}(a^i, x^{-i}_{s, n})$, $\hat beta_{s, n}$ is the update rate and other notations are those of our paper.

Since the estimate are per state-action and not only per state (as in our work) it is possible to use a model-free update rule where the transition is not needed:

\optmult{\hat Q_{i, s, n}(a) = \hat Q_{i, s, n}(a) \\ + \hat \beta_{s, n}\left(r^i(s, a) + \gamma v_{i, n}(s')-\hat Q_{i, s, n}(a)\right)}
where $s'$ is the next state.

Therefore, the state transition is implicitly estimated in the model-free version of the algorithm in the $Q$-function, as long as there is an infinite number of times when the system is in state $s$ and every action $a$ is played. A similar mechanism would be interesting for our procedure: we cannot directly use the same idea as our state-value estimate $u_{s, n}$ (which is the analog of $Q_{i, s, n}$) is not per action.

\paragraph{Fictitious play in multi-stage games}
\citeauthor*{perolatActorcriticFictitiousPlay2018} proposed a fictitious play process for multistage games \cite{perolatActorcriticFictitiousPlay2018}. In multi-stage games, states can be naturally ordered as a tree with an initial state and a final state, an assumption that we do not make. 
The fact that states are ordered as a tree is helpful to do proofs by inductions but covers a smaller class of games. There is nevertheless common features between our procedure and the procedure outlined in \cite{perolatActorcriticFictitiousPlay2018}.

Technically, it involves the estimation of a state-action value function $Q^i_{n}(s, a)$ where $i$ is a player, $s$ the state, $a$ the action and $n$ the update step of the algorithm and the computation of a strategy where the probablity for player $i$ to play $a$ in state $s$ at step $n$ is $\pi^i_n(s, a)$. 

Values $\pi^i_n(s, a)$ is updated towards a logit-choice best-response with regards to the current state-action value function $Q^i_{n}(s, a)$. This is a difference with our procedure which uses a plain best-response that are potentially non-unique, hence the need for differential inclusions (which are not needed for \citeauthor*{perolatActorcriticFictitiousPlay2018}). Our procedure is also simpler to implement (it is not necessary to use a logit function) and interesting from an epistemic point of view in game theory (players take a best response without randomness).

Values $Q^i_n(s, a)$ are updated towards an iterate of the Bellman operator (either using the current strategy or using the logit-choice best-response strategy). In contrast, our procedure updates state-values which is presumably a smaller set of estimates but require either the transition matrix or an estimation of these transitions.

In \cite{perolatActorcriticFictitiousPlay2018}, other players strategy are not observed. In our paper, we model every player independently in a similar way as fictitious play of \citeauthor*{brown1951iterative} and \citeauthor{robinsonIterativeMethodSolving1951}. This can be seen as a limitation of our work since it requires more information during the play. However, we believe that a more precise model of players can be interesting for two reasons. First, from a general perspective, it is interesting to study models where more information about the environment is known because it makes it possible to converge to sets that may not be attainable in more relaxed settings \cite{hartSimpleAdaptiveProcedure2000a}. Second, we believe it can converge faster in the appropriate environment (especially with a large number of players), even if we lack theoretical or experimental evidence. It would be interesting to compare our algorithm to the one outlined in \citeauthor{perolatActorcriticFictitiousPlay2018}.
