# Supplementary material for: Best-Response Dynamics and Fictitious Play in Identical-Interest and Zero-Sum Stochastic Games
Source: arXiv:2111.04317 source file (2022-05-16)
Supplement: Supplementary file 2 [file appendix_strongly_async.tex]

\hypertarget{convergence-of-the-asynchronous-system}{%
\paragraph{Convergence of the asynchronous
system}\label{convergence-of-the-asynchronous-system}}

We now suppose that \(\delta \in (0, 1/|S|)\). In what follows \(\{u^i_s, x^i_s\}_{s\in \states, i \in I}\) is a
solution of \ref{eq:abrd} for identical interest stochastic games.
\GV{Manque le numero}
We use the same definitions for $\optgap$ and $\payt s t$:
\[\begin{aligned}\payt s t := &\stfs \cut {x_s(t)} \\ \optgap := & \max\limits_{y \in A^i} \stfs \cut {y, \cxs {-i} t} - \stfs \cut {\cxs {} t} \\ = & \max\limits_{y \in A^i} \stfs \cut {y, \cxs {-i} t} - \payt s t\end{aligned}\]

\iffalse
\begin{lemma}\label{afp:paydiff}

Function \(\pay s: t \mapsto \stfs \cut {x_s(t)}\) is
differentiable and:
\[\dfrac{d\pay s}{dt} = \delta \sum_{s'} \ratest {s'} t P_{s s'}(x_s)\dot u_{s'} + \ratest s t \sum_i \optgap\]\end{lemma}

\begin{proof}
The proof is the same as Lemma \ref{lem:diffgamma} but with $\beta_s$.
\end{proof}
\fi

We now define $\paysup$ which measures how much the estimated payoffs $u_s$ are over estimated compared to $\payt s t$:

\begin{align*}\paysup(t) & = \sum_{s\in \states} \pos{u_s(t) - \payt s t} \\ & = \sum_{s \in \states} 1_{u_s - \payt s t \geq 0}(u_s(t) - \payt s t)\end{align*}

\begin{lemma}\label{lem:convabrd}

For a solution \(\{u_s, x^i_s, \beta_s\}_{i \in I, s \in \states}\) of
\ref{eq:abrd}:

\begin{itemize}
\item
  \(\paysup(t) \leq \paysup(1)\exp\left(\int_1^t (\delta|S|-1)\frac{\beta_-}{\crateu u}du\right)\iffalse = \paysup(1)t^{\delta|S|-1}\fi\)
\item
  every \(u_s\) converges
\item
  every \(\pay s\) converges
\item
  the limits of \(u_s\) and \(\pay s\) are the same.
\end{itemize}

\end{lemma}

\begin{proof}

First, for readability, we pose $1_s(t) := 1_{u_s-\payt s t > 0}$.

\newcommand{\ones}[1]{1_{#1}(t)}

\(\paysup\) is continuous and differentiable almost everywhere (if there
is an accumulation point where for a \(s\), \(u_s(t) - \payt s t = 0\),
then \(\diff {} {(u_s-\pay s)} = 0\), so
\(1_{u_s(t) - \payt s t\geq 0} (u_s-\pay s)\) is differentiable and its
derivative is \(0\)).
:{\small
\begin{equation}
  \begin{aligned}
    \diff \paysup & = \sum_{s\in \states} \ones s \left(
      \begin{aligned}
        \ratest s t \frac{\payt s t - u_s(t)}{\crateu {\int_0^t \ratest s u du} }- \ratest s t \sum_i \optgap \\
        - \delta \sum_{s'} P_{s s'}(x_s) \ratest {s'} t \frac{\payt {s'} t - u_{s'}(t)}{\crateu {\int_0^t \ratest {s'} u du} }
      \end{aligned}\right)\\
    & \leq \sum_{s\in \states} \ones s \left(
      \begin{aligned}
        &\ratest s t \frac{\payt s t - u_s(t)}{\crateu {\int_0^t \ratest s u du} } \\
        &- \delta \sum_{s'} P_{s s'}(x_s) \ratest {s'} t \frac{\payt {s'} t - u_{s'}(t)}{\crateu {\int_0^t \ratest {s'} u du} }
      \end{aligned}\right)\\
    & = \sum_{s \in \states} \left(
      \begin{aligned}
        \ones s \\
        - \delta \sum_{s'} \ones {s'} P_{s' s}(x_{s'})
      \end{aligned}\right) \ratest s t \frac{\payt s t - u_s(t)}{\crateu {\int_0^t \ratest s u du} }\end{aligned}\end{equation}}

\begin{itemize}
  \item If \(u_s(t) - \payt s t < 0\), then the summed term is equal to
        \(- \delta \sum_{s'} \ones {s'} P_{s's}(x_{s'}) \ratest s t \frac{\payt s t - u_s(t)}{\crateu {\int_0^t \ratest s u du} } \leq 0\). Since \((u_s(t) - \payt s t)_+=0\), the summed term is lower than: $$-(1-\delta|S|)\frac{\beta_-}{\alpha(t)}\pos{u_s(t)-\payt s t}$$
  \item  If \(u_s(t) - \payt s t > 0\), then the summed term is equal to
        \(\left(1 - \delta \sum_{s'} \ones {s'}  P_{s's}(x_{s'})\right) \ratest s t \frac{\payt s t - u_s(t)}{\crateu {\int_0^t \ratest s u du} }\)

        \begin{itemize}
          \item \(\delta \sum_{s'} \ones {s'} P_{s's}(x_{s'}) \leq \delta |S| < 1\)
          \item so \(1 - \delta \sum_{s'} \ones {s'} P_{s's}(x_{s'}) > 0\).
          \item so \(\left(1 - \delta \sum_{s'} \ones{s'} P_{s's}(x_{s'})\right) \ratest s t \frac{\payt s t - u_s(t)}{\crateu {\int_0^t \ratest s u du} } < 0\)
          \item but $\ratest s t \geq \beta_-$ and $\crateu {\int_0^t \ratest s u du} \leq \crateu t$, \newline so $\frac{\ratest s t}{\crateu {\int_0^t \ratest s u du}} \geq \frac{\beta_-}{\crateu t}$
          \item so the summed term is lower than: \begin{multline*}(1-\delta|S|)\frac{\beta_-}{\crateu t}(\payt s t - u_s(t)) \\= - (1-\delta|S|)\frac{\beta_-}{\crateu t}\pos{u_s(t) - \payt s t}\end{multline*}
        \end{itemize}
\end{itemize}

\iffalse

In the second case,
\(\left(1 - \delta \sum_{s'} 1_{u_{s'}-\payt {s'} t > 0} P_{s's}(x_{s'})\right) \ratest s t \frac{\payt s t - u_s(t)}{\crateu {\int_0^t \ratest s u du} } < (1-\delta |S|)\frac{\beta_{-}}{\crateu t} (\payt s t - u_s(t))\).

And if \(u_s(t) - \payt s t > 0\), then
\(\payt s t - u_s(t) = - \pos{u_s(t) - \payt s t}\), so
\(\diff \paysup \leq -(1-\delta |S|)\frac{\beta_-}{\crateu t}\paysup(t)\)
\fi

Consequently:
\[\diff \paysup \leq -(1-\delta |S|)\frac{\beta_-}{\crateu t}\paysup(t)\]

So by Grönwall Lemma (see Lemma \ref{ineqgu} for the details of the
application of Grönwall Lemma):

\[\paysup(t) \leq \paysup(1)\exp\left(\int_1^t -(1-\delta|S|)\frac{\beta_-}{\crateu u}du\right)\iffalse = \paysup(1)t^{\delta|S|-1}\fi\]

So $\paysup$ goes to $0$ when $t$ goes to $+\infty$ because of Hypothesis~\eref{eq:alpha}.

Now we lower bound $\diff {u_s}$ to show convergence of $u_s$.

\[\begin{aligned}\diff {u_s} = & \ratest s t \frac{\payt s t - u_s(t)}{\int \ratest s u du} \\ \geq & \ratest s t \frac{-\paysup(t)}{\crateu {\int \ratest s u du}} \\ \geq & -\psi(1)\frac{\exp\left(\int_1^t -(1-\delta|S|)\frac{\beta_-}{\crateu u}du\right)}{\crateu{\int \ratest s u du}} \\ \geq & -\psi(1)\frac{\exp\left(\int_1^t -(1-\delta|S|)\frac{\beta_-}{\crateu {\int \ratest s u du}}du\right)}{\crateu{\int \ratest s u du}}\end{aligned}\]

As \(\delta|S| < 1\), this last term is integrable, therefore, as
\(u_s\) is bounded, this means that \(u_s\) converges. The same argument
applies to \(\pay s\) using Lemma~\ref{lem:diffgamma}, and the limits of
\(u_s\) and \(\pay s\) are necessarily the same (otherwise the
derivative of \(u_s\) converge towards
\(\frac{\lim u_s - \lim \pay s}{\crateu t}\) which would result in a diverging
\(u_s\)).\end{proof}

\begin{lemma} The gap between $\payt s t$ and $\max_{y\in A^i}\stfs {u(t)}{y, x^{-i}_s(t)}$ converges to 0:
  \[\forall s, \sum_i \optgap \rightarrow 0\]
  \label{lem:delta0async}\end{lemma}

\begin{proof}
The proof proceeds similarly to Lemma~\ref{lem:delta0}.
First, we show that \(\forall i,s\),
\(\int_1^\infty \sum_{i\in I} \optgap dt < + \infty\).

From Lemma~\ref{lem:diffgamma},
\(\ratest s t \sum_i \optgap = \frac{d\pay s}{dt} - \delta \sum_{s'} P_{s s'}(x_s)\dot u_s\).
Then:
\[\forall T, \int_1^T\sum_i \ratest s t \optgap dt = \int_1^T \frac{d\pay s}{dt} - \delta\sum_{s'}\int_1^TP_{ss'}(x_s)\dot u_s\]

With the previous lemma:
\[\begin{aligned}P_{ss'}(x_s)\dot u_s & = P_{ss'}(x_s) \ratest {s'} t  \dfrac{\payt s t-u_s(t)}{\crateu {\int_0^t \ratest s v dv}} \\ & \geq -P_{ss'}(x_s) \frac{\paysup(t)}{\int_0^t \ratest s v dv}\end{aligned}\]

(because $\ratest s t \leq 1$ and $\payt s t - u_s(t) \geq - \pos{u_s(t) - \payt s t}$).

Then, for all $T$:
{ \[
  \begin{aligned}
    \beta_- \int_1^T\sum_i \optgap dt 
    & \leq \int_1^T\sum_i \ratest s t \optgap dt \\ &\leq \payt s T - \payt s 1\\
    & + \delta\sum_{s'}P_{ss'}(x_s)\int_1^T \paysup(1)\dfrac{\exp\left(\int_1^t \frac{\delta|S|-1}{\crateu v}dv\right)}{\crateu {\int_0^t \ratest s v dv}}\\&=\payt s T-\payt s 1 \\
    & + \delta\sum_{s'}\int_1^T \paysup(1)\dfrac{\exp\left(\int_1^t \frac{\delta|S|-1}{\crateu {\int_0^t \ratest s w dw}}dv\right)}{\crateu {\int_0^t \ratest s v dv}}\\&=\payt s T-\payt s 1 \\
    &  + \delta\frac{A}{\delta-1} \left(\exp\left(\int_1^T \frac{\delta-1}{\crateu {\int_0^t \ratest s v dv}}\right)-1\right)\\
    & <\payt s T-\payt s 1 + \delta\frac{A}{1-\delta}
  \end{aligned}\]}

Then, as $\optgap$ is Lipschitz (Lemma~\ref{lem:deltalip}) and the limit of its integral is bounded and
positive, \(\optgap \limt 0\).\end{proof}

\begin{proof}[Proof of the part about~\ref{eq:abrd} of Theorem~\ref{thm:contasync}]
\ \newline 
It is Lemma~\ref{lem:convabrd} and the same proof as Lemma~\ref{lem:contconvequilibria}.

\end{proof}
